# Supplementary material for: Weak Links in Authentication Chains: A Large-scale Analysis of Email Sender Spoofing Attacks
Source: arXiv:2011.08420 source file (2020-11-17)
Supplement: Supplementary file 1 [file appendix.tex]

\section{Changes for Major Revision}
This paper receives a Major Revision decision in the Fall Quarter of USENIX Security '20. We appreciate all reviewers for their valuable comments, which significantly help us improve. According to the reviewers’ advice, we made the following changes to improve this paper.

\myparagraph{Improvements in writing and presentation}
We made great efforts to improve writing and presentation performance of this study. First, we adopted the recommendation of reviewer D and reorganized the structure of the paper. We divided the attacks into four categories by different stages of the email delivery process. Second, we presented both the attacks and its target in smaller groups so that readers can keep track of these in section ~\ref{email_attacks}. Third, we also modified the description of each attack method and added relevant diagrams and figures to explain workflows in detail. Finally, we polished the text and fixed the language problems in the last version.

\myparagraph{Methodology about the vulnerability discovery process}
We add the descriptions about the vulnerability discovery methodology in section ~\ref{methodology}. 
First, we systematically analyzed email specifications and extracted the ABNF rules, focusing on headers related to authentication, such as \texttt{Mail From/From/Helo/Sender} headers. 
Second, we generated our test samples based on the ABNF grammar for the authentication-related headers. Third, we introduced the common mutation methods in the protocol fuzz, such as header repeating, inserting spaces, inserting Unicode characters, header encoding, and case variation.
Fourth, we used a four-stage method to test the security verification logic of the target email systems with our generated samples. 
Finally, we analyzed and summarized the employed adversarial techniques that make email sender spoofing successful in practice. Throughout the process, we considered the possible security risks of all Unicode characters.

\myparagraph{Novelty of attacks}
This study systematically analyzed the transmission process of an email. We have investigated a total of 14 email spoofing attacks, of which 9(e.g., A$_3$, A$_6$, A$_7$ and etc.) are new attacks, to best of our knowledge so far. 
%For example, no one mentioned before whether the security risk brought by adding DKIM signatures in mail forwarding. The DKIM signature fraud(A$_{11}$ attack is undoubtedly novel.

\myparagraph{Benefits of combined attacks}
% Email system is a complex ecosystem with multi-party trust chain, which rely on security measures implemented and deployed by multiple parties. As a result, email authenticity depends on the weakest link in the email authentication chain. 
One attack alone may not achieve the intended forgery effect. A combined attack, however, is far more effective than simply adding their respective power.
As discussed in the paper, the DKIM signature fraud attack(A$_{11}$ will deceive a legitimate DKIM signature, but it still needs the cooperation of other attacks(e.g., A$_2$, A$_3$) to completely bypass SPF, DKIM, DMARC and user-interface protections. Furthermore, the effectiveness of a combined attack reveals the vulnerability of this chain-based authentication structure in the email ecosystem. Any fragile part can break the whole authentication chain. And the detail is discussed in section ~\ref{combined_attacks}.

\myparagraph{Supplement the work of the email client.}
Thanks to reviewers' suggestions, we added experiments on 23 popular email clients to measure the impact of our attacks in different operating systems. Table ~\ref{tab:client_results1} shows that almost all email clients are vulnerable to the various attacks we found in the UI rendering stage. For example, the famous email client, Outlook, is vulnerable to the attacks A$_7$ and A$_{15}$. We think this is a new contribution after major revision.

\myparagraph{The difference between our work and Hang Hu's work }
Hang Hu and Gang Wang\cite{hu2018end} did a spoofing experiment in 2018, using only the most basic spoofing method with a faked \texttt{Mail From} header. Their work did not concentrate on bypassing validation of SPF, DKIM or DMARC. They found that many email providers would still allow the delivery of emails as long as the policy of the spoofed domain is not very strict(“reject”).
Moreover, most of such vulnerabilities have been fixed in the past two years. 

Our study focuses on new attack methods to bypass protocol verification or user-interface protections. In addition, the target legitimate domain has deployed more strict "reject" policy for SPF or DMARC in our experiment.
We reproduced the same experiment\cite{hu2018end} to test 30 popular email services. The results show that 23 email services will reject emails because of failure to pass SPF, DKIM and DMARC verification. The remaining 7 email services will put them in the spam folder. In contrast, with our new attacks, attacker can forge spoofing email successfully to bypass all protections.

\myparagraph{An improved Discussion section}
In this version, we replace the Discussion section with Root Causes and Mitigation ~\ref{discussion}. We explored the scope and root causes of these attacks we found. We think these attacks share the high-level theme that the inconsistency among multiple parties' understanding and implementation of security mechanisms, which has led to more security issues. One party(e.g., sender) alone might implement the security mechanisms correctly; but when integrated into a larger system, it is still venerable to a variety of attacks,  especially the combined attacks.  

\myparagraph{Modifications to the previous version of Table 2 and 3}
Reviewers think that Table 2 and 3 are ambiguous in the last edition, so we redesigned the tables to show the experiment results and added additional findings of corporate email clients. Now Table ~\ref{tab:experiment_results1} shows the sender spoofing experiment results on 30 target mail services and Table ~\ref{tab:client_results1} shows the results on 23 target  email clients. In section ~\ref{results}, we further explained the two tables in details.

\myparagraph{Ethics of our experiment}:
We added an ethics description in section ~\ref{experiment_setup}. In the experiments, we only use dedicated email accounts owned by ourselves. No real users are affected by our experiments. We have also carefully controlled the message sending rate with intervals over 10 minutes to minimize the impact on the target email services.
